# Supplementary material for: A force field of Li$^+$ , Na$^+$ , K$^+$, Mg$^{2+}$, Ca$^{2+}$, Cl$^-$, and SO$_4^{2-}$ in aqueous solution based on the TIP4P/2005 water model and scaled charges for the ions
Source: arXiv:2401.13164 source file (2024-01-24)
Supplement: Supplementary file 1 [file supplementary_force_field_madrid_carlos.pdf]

## Supplementary material

### A force field of $\text{Li}^+$ , $\text{Na}^+$ , $\text{K}^+$ , $\text{Mg}^{2+}$ , $\text{Ca}^{2+}$ , $\text{Cl}^-$ , and $\text{SO}_4^{2-}$ in aqueous solution based on the TIP4P/2005 water model and scaled charges for the ions

I. M. Zeron, J. L. F. Abascal, and C. Vega

*Depto. Química Física I, Fac. Ciencias Químicas, Universidad  
Complutense de Madrid, 28040 Madrid, Spain*

Here are presenting all the results of this work in tabular form so that they can be reproduced.

TABLE I. Comparison between Lennard-Jones parameters for NaCl solutions in TIP4P/2005 water for the previous NaCl model (Madrid model<sup>1</sup>) and the current model (Madrid-2019 model). Changes are highlighted.

| Interaction               | Madrid model              |                                 | Madrid-2019 model         |                                 |
|---------------------------|---------------------------|---------------------------------|---------------------------|---------------------------------|
|                           | $\sigma_{LJ}/(\text{nm})$ | $\epsilon_{LJ}/(\text{kJ/mol})$ | $\sigma_{LJ}/(\text{nm})$ | $\epsilon_{LJ}/(\text{kJ/mol})$ |
| $\text{Na}^+-\text{Na}^+$ | 0.221 737                 | 1.472 356                       | 0.221 737                 | 1.472 356                       |
| $\text{Cl}^--\text{Cl}^-$ | 0.484 906                 | 0.076 923                       | <b>0.469 906</b>          | 0.076 923                       |
| $\text{Na}^+-\text{Cl}^-$ | 0.290 512                 | 1.438 894                       | <b>0.300 512</b>          | 1.438 894                       |
| O-O                       | 0.315 890                 | 0.774 908                       | 0.315 890                 | 0.774 908                       |
| $\text{Na}^+-\text{O}$    | 0.251 338                 | 0.793 388                       | <b>0.260 838</b>          | 0.793 388                       |
| $\text{Cl}^--\text{O}$    | 0.426 867                 | 0.061 983                       | <b>0.423 867</b>          | 0.061 983                       |

TABLE II. Madrid-2019 simulation results for density and shear viscosity as were obtained for LiCl solutions in TIP4P/2005 water at temperature  $T = 298.15$  K and pressure  $P = 1$  bar for different concentrations below experimental solubility. Numbers in parentheses are de uncertainty in the results. Data in the Expt columns are from our fit of experimental data taken from Refs. 2–4 and references therein.

| Molality<br>(mol/Kg) | Density<br>(Kg/m <sup>3</sup> ) |           | Viscosity<br>(mPa s) |      |
|----------------------|---------------------------------|-----------|----------------------|------|
| m                    | Expt                            | Sim       | Expt                 | Sim  |
| 0.0                  | 997.047                         | 997.3     | 0.89                 | 0.88 |
| 0.5                  | 1009.0                          | 1008.3(5) |                      |      |
| 1.0                  | 1020.5                          | 1018.9(5) |                      |      |
| 3.0                  | 1062.1                          | 1059.1(5) | 1.32                 | 1.71 |
| 6.0                  | 1115.5                          | 1114.6(5) | 1.93                 | 3.05 |
| 9.0                  | 1162.2                          | 1165.4(5) |                      |      |
| 12.0                 | 1204.3                          | 1213.0(5) | 7.54                 | 17   |

TABLE III. As in Table II for NaCl solutions.

| Molality<br>(mol/Kg) | Density<br>(Kg/m <sup>3</sup> ) |           | Viscosity<br>(mPa s) |      |
|----------------------|---------------------------------|-----------|----------------------|------|
| m                    | Expt                            | Sim       | Expt                 | Sim  |
| 0.0                  | 997.047                         | 997.3     | 0.89                 | 0.88 |
| 0.5                  | 1017.10                         | 1017.3(5) |                      |      |
| 1.0                  | 1036.21                         | 1036.2(5) | 0.97                 | 1.05 |
| 2.0                  | 1072.27                         | 1072.5(5) | 1.07                 | 1.27 |
| 3.0                  | 1105.76                         | 1105.8(5) |                      |      |
| 4.0                  | 1136.91                         | 1137.3(5) | 1.35                 | 1.75 |
| 5.0                  | 1165.91                         | 1166.9(5) |                      |      |
| 6.0                  | 1192.88                         | 1194.6(5) |                      |      |

TABLE IV. As in Table II for KCl solutions.

| Molality<br>(mol/Kg) | Density<br>(Kg/m <sup>3</sup> ) |           | Viscosity<br>(mPa s) |      |
|----------------------|---------------------------------|-----------|----------------------|------|
| m                    | Expt                            | Sim       | Expt                 | Sim  |
| 0.0                  | 997.047                         | 997.3     | 0.89                 | 0.88 |
| 0.5                  | 1019.8                          | 1020.1(5) |                      |      |
| 1.0                  | 1041.4                          | 1041.8(5) | 0.89                 | 0.94 |
| 2.0                  | 1081.5                          | 1082.0(5) | 0.90                 | 1.03 |
| 3.0                  | 1118.3                          | 1119.0(5) |                      |      |
| 4.0                  | 1152.2                          | 1152.8(5) | 0.94                 | 1.22 |
| 4.5                  | 1168.2                          | 1168.8(5) |                      |      |

TABLE V. As in Table II for  $\text{MgCl}_2$  solutions.

| Molality<br>(mol/Kg) | Density<br>(Kg/m <sup>3</sup> ) |           | Viscosity<br>(mPa s) |      |
|----------------------|---------------------------------|-----------|----------------------|------|
| m                    | Expt                            | Sim       | Expt                 | Sim  |
| 0.0                  | 997.047                         | 997.3     | 0.89                 | 0.88 |
| 0.1                  | 1004.9                          |           | 0.91                 | 0.98 |
| 0.5                  | 1035.0                          | 1033.5(5) | 1.07                 |      |
| 1.0                  | 1070.3                          | 1067.8(5) | 1.34                 | 1.42 |
| 2.0                  | 1135.4                          | 1132.6(5) | 1.92                 |      |
| 3.0                  | 1194.1                          | 1192.7(5) | 2.95                 | 4.4  |
| 4.0                  | 1246.7                          | 1248.6(5) | 4.79                 |      |
| 5.0                  | 1295.5                          | 1302.3(5) | 7.77                 | 16   |

TABLE VI. As in Table II for  $\text{CaCl}_2$  solutions.

| Molality<br>(mol/Kg) | Density<br>(Kg/m <sup>3</sup> ) |           | Viscosity<br>(mPa s) |      |
|----------------------|---------------------------------|-----------|----------------------|------|
| m                    | Expt                            | Sim       | Expt                 | Sim  |
| 0.0                  | 997.047                         | 997.3     | 0.89                 | 0.88 |
| 0.1                  |                                 |           | 0.92                 | 0.92 |
| 0.5                  | 1041.0                          | 1041.2(5) | 1.03                 | 1.07 |
| 1.0                  | 1082.2                          | 1082.5(5) | 1.19                 | 1.37 |
| 2.0                  | 1157.8                          | 1157.1(5) |                      |      |
| 3.0                  | 1225.9                          | 1222.9(5) | 2.24                 | 2.97 |
| 4.0                  | 1287.4                          | 1280.0(5) |                      |      |
| 5.0                  | 1342.4                          | 1329.3(5) | 4.92                 | 9.10 |
| 6.0                  | 1390.7                          | 1371.5(5) |                      |      |

TABLE VII. As in Table II for  $\text{Li}_2\text{SO}_4$  solutions.

| Molality<br>(mol/Kg) | Density<br>(Kg/m <sup>3</sup> ) |           | Viscosity<br>(mPa s) |      |
|----------------------|---------------------------------|-----------|----------------------|------|
| m                    | Expt                            | Sim       | Expt                 | Sim  |
| 0.0                  | 997.047                         | 997.3     | 0.89                 | 0.88 |
| 0.5                  | 1042.0                          | 1040.9(5) |                      |      |
| 1.0                  | 1083.6                          | 1080.7(5) |                      |      |
| 1.5                  | 1122.2                          | 1117.4(5) | 1.97                 | 1.63 |
| 2.0                  | 1158.2                          | 1151.3(5) |                      |      |
| 2.5                  | 1192.1                          | 1182.8(5) |                      |      |
| 3.0                  | 1224.4                          | 1212.1(5) | 4.39                 | 2.92 |

TABLE VIII. As in Table II for  $\text{Na}_2\text{SO}_4$  solutions.

| Molality<br>(mol/Kg) | Density<br>(Kg/m <sup>3</sup> ) |           | Viscosity<br>(mPa s) |      |
|----------------------|---------------------------------|-----------|----------------------|------|
| m                    | Expt                            | Sim       | Expt                 | Sim  |
| 0.0                  | 997.047                         | 997.3     | 0.89                 | 0.88 |
| 0.5                  | 1057.3                          | 1057.9(5) | 1.10                 | 1.00 |
| 1.0                  | 1112.4                          | 1112.3(5) | 1.37                 | 1.19 |
| 1.5                  | 1163.8                          | 1162.6(5) | 1.73                 | 1.58 |

TABLE IX. As in Table II for  $\text{K}_2\text{SO}_4$  solutions.

| Molality | Density              |           | Viscosity |       |
|----------|----------------------|-----------|-----------|-------|
| (mol/Kg) | (Kg/m <sup>3</sup> ) |           | (mPa s)   |       |
| m        | Expt                 | Sim       | Expt      | Sim   |
| 0.0      | 997.047              | 997.3     | 0.89      | 0.88  |
| 0.1      | 1010.8               | 1011.3(5) | 0.91      | 0.875 |
| 0.2      | 1024.1               | 1024.6(5) |           |       |
| 0.25     | 1030.7               | 1031.0(5) | 0.94      | 0.88  |
| 0.4      | 1049.9               | 1050.0(5) |           |       |
| 0.5      | 1062.4               | 1062.6(5) | 0.99      | 0.92  |
| 0.6      | 1074.7               | 1074.4(5) |           |       |

TABLE X. As in Table II for  $\text{MgSO}_4$  solutions.

| Molality | Density              |           | Viscosity |      |
|----------|----------------------|-----------|-----------|------|
| (mol/Kg) | (Kg/m <sup>3</sup> ) |           | (mPa s)   |      |
| m        | Expt                 | Sim       | Expt      | Sim  |
| 0.0      | 997.047              | 997.3     | 0.89      | 0.88 |
| 0.5      | 1055.1               | 1054.5(5) |           |      |
| 1.0      | 1109.6               | 1107.3(5) |           |      |
| 1.5      | 1161.4               | 1157.1(5) | 2.42      | 1.74 |
| 2.0      | 1209.9               | 1203.4(5) |           |      |
| 2.5      | 1255.9               | 1247.0(5) | 5.15      | 2.98 |

<sup>1</sup> A. L. Benavides, M. A. Portillo, V. C. Chamorro, J. R. Espinosa, J. L. F. Abascal, and C. Vega, J. Chem. Phys. **147**, 104501 (2017).

<sup>2</sup> M. Laliberte and W. E. Cooper, J. Chem. Eng. Data **49**, 1141 (2004).

<sup>3</sup> M. Laliberté, J. Chem. Eng. Data **52**, 321 (2007).

<sup>4</sup> M. Laliberté, J. Chem. Eng. Data **54**, 1725 (2009).
